# Supplementary material for: Divide and Conquer Dynamic Programming: An Almost Linear Time Change Point Detection Methodology in High Dimensions
Source: arXiv:2301.10942 source file (2023-06-02)
Supplement: Supplementary file 1 [file 99_appendix.tex]

\section{Detail of algorithms}
\label{sec:dp}

The $\ell_0$ penalization approach considers the joint optimization problem
\begin{equation}
    \hat{\mclP} = \argmin_{\mclP} \left\lbrace \sum_{I\in \mclP} L(\hat{\theta}(\mclI),\mclI) + \gamma |\mclP| \right\rbrace, \quad \hat{\theta}(\mclI) = \argmin_{\theta} L(\theta,\mclI),
    \label{eq:P_hat_high_dim}
\end{equation}
where $\mclP$ is a collections of points in $(0,T]$ and for any interval $\mclI = (s,e]$, $\mclI\in \mclP$ means $\{s,e\}\in \mclP$. If we put the constraint $|\mclP|\leq K$, then a brute-force search can find the global minimizer $\hat{\mclP}$ with $O(T^K)$ time complexity. For a given $\gamma$, it can be seen that $|\hat{\mclP}|\leq \frac{1}{\gamma}L(\hat{\theta}((0,T]),(0,T])$. Instead, by the dynamic programming algorithm \ref{algorithm:DP} with grid $[T]$, we can solve \eqref{eq:P_hat_high_dim} with $T^2$ complexity, which is free of parameter $\gamma$.





\section{Additional Experiments}
\label{sec:add_experiment}


\subsection{Selection of $\gamma$}
In the theory of DCDP, we need $\gamma = C_{\gamma}K\tr$, which is increasing with $\Delta$. If $\gamma$ gets smaller, it's more likely that the DP will select more false positive change points. In experiments, we can observe a similar phenomenon: in \Cref{fig:small_big_gamma}, the localization error using CV list of $\gamma$ with bigger values is smaller than that using CV list with smaller values.

The next question is, if we include both small and big values of $\gamma$ in the CV list, can the algorithm pick the big values by itself? The answer is NO. \Cref{fig:pick_gamma} shows the best gamma that selected by the CV step, and there is no clear pattern for selecting bigger $\gamma$. On the other hand, \Cref{fig:error_gamma} shows that bigger $\gamma$ indeed leads to better localization error. Therefore, in conclusion, we do need bigger $\gamma$ for DCDP, but the algorithm itself cannot pick bigger $\gamma$ from a wide range: what we can do is to manually set a CV list of $\gamma$ with big values.

\begin{figure}[H]
    \centering
    \includegraphics[width = 0.92 \textwidth]{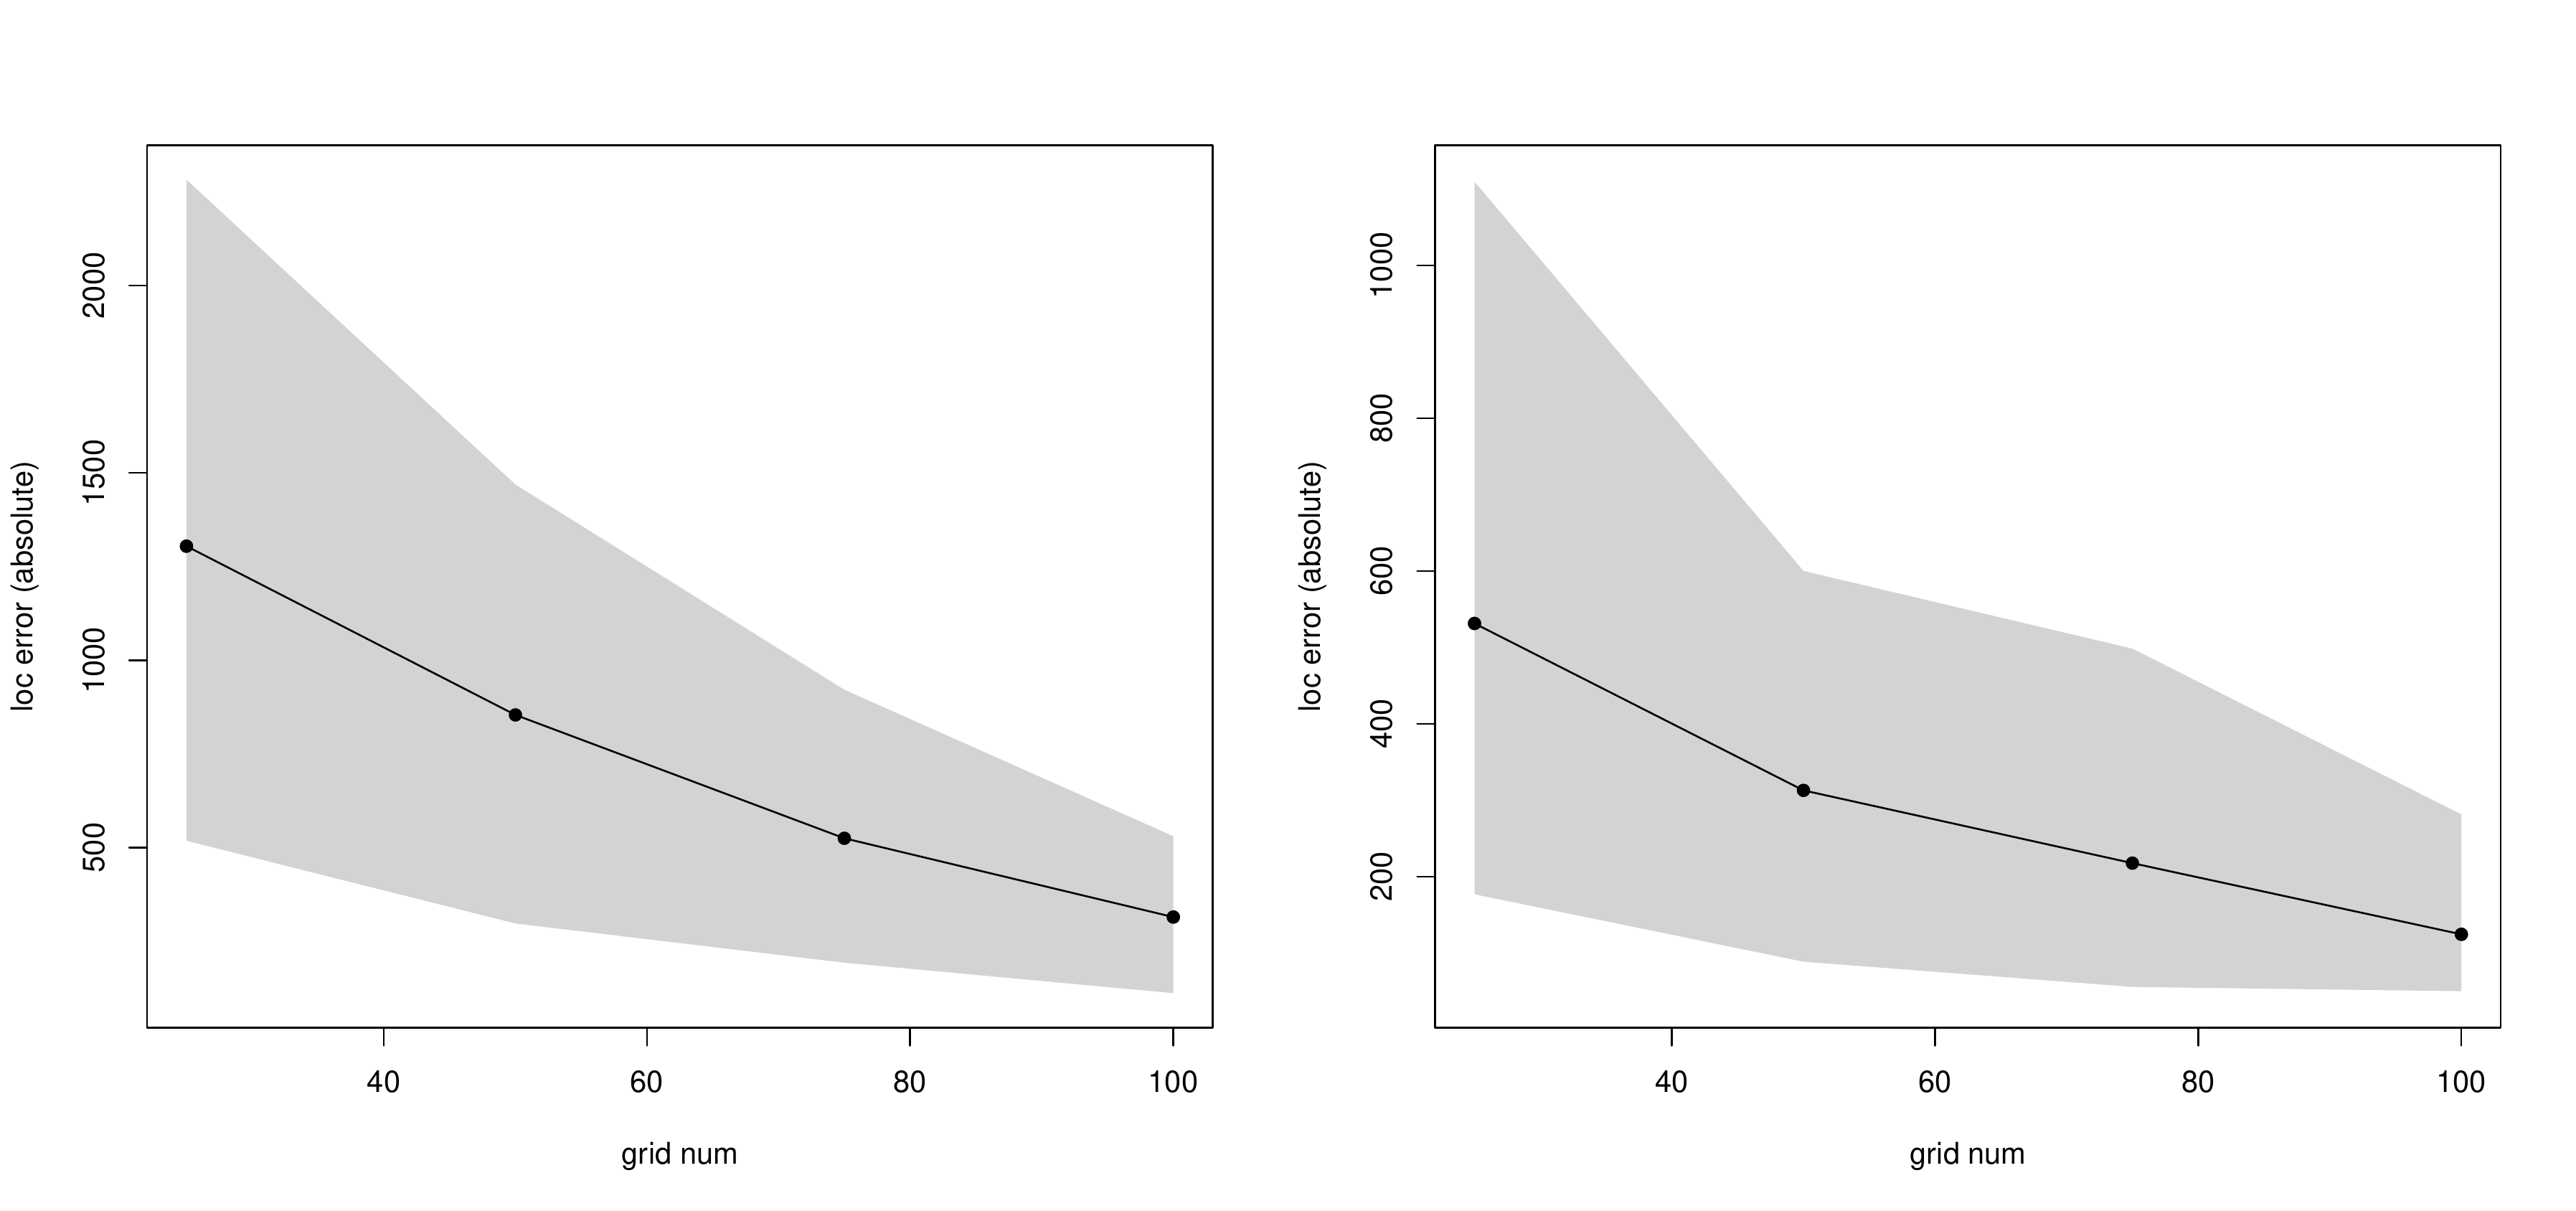}
    \caption{Localization error vs. $\mclQ$ with $\Delta = 5000$. Left: the CV list of $\gamma$ is $\{10, 20, 40, 80\}$; right: the CV list of $\gamma$ is $\{1000,2000,3000\}$. The line is the average and the shaded area shows the upper and lower 0.1 quantiles from 60 trials.}
    \label{fig:small_big_gamma}
\end{figure}

\begin{figure}[H]
    \centering
    \includegraphics[width = 0.92 \textwidth]{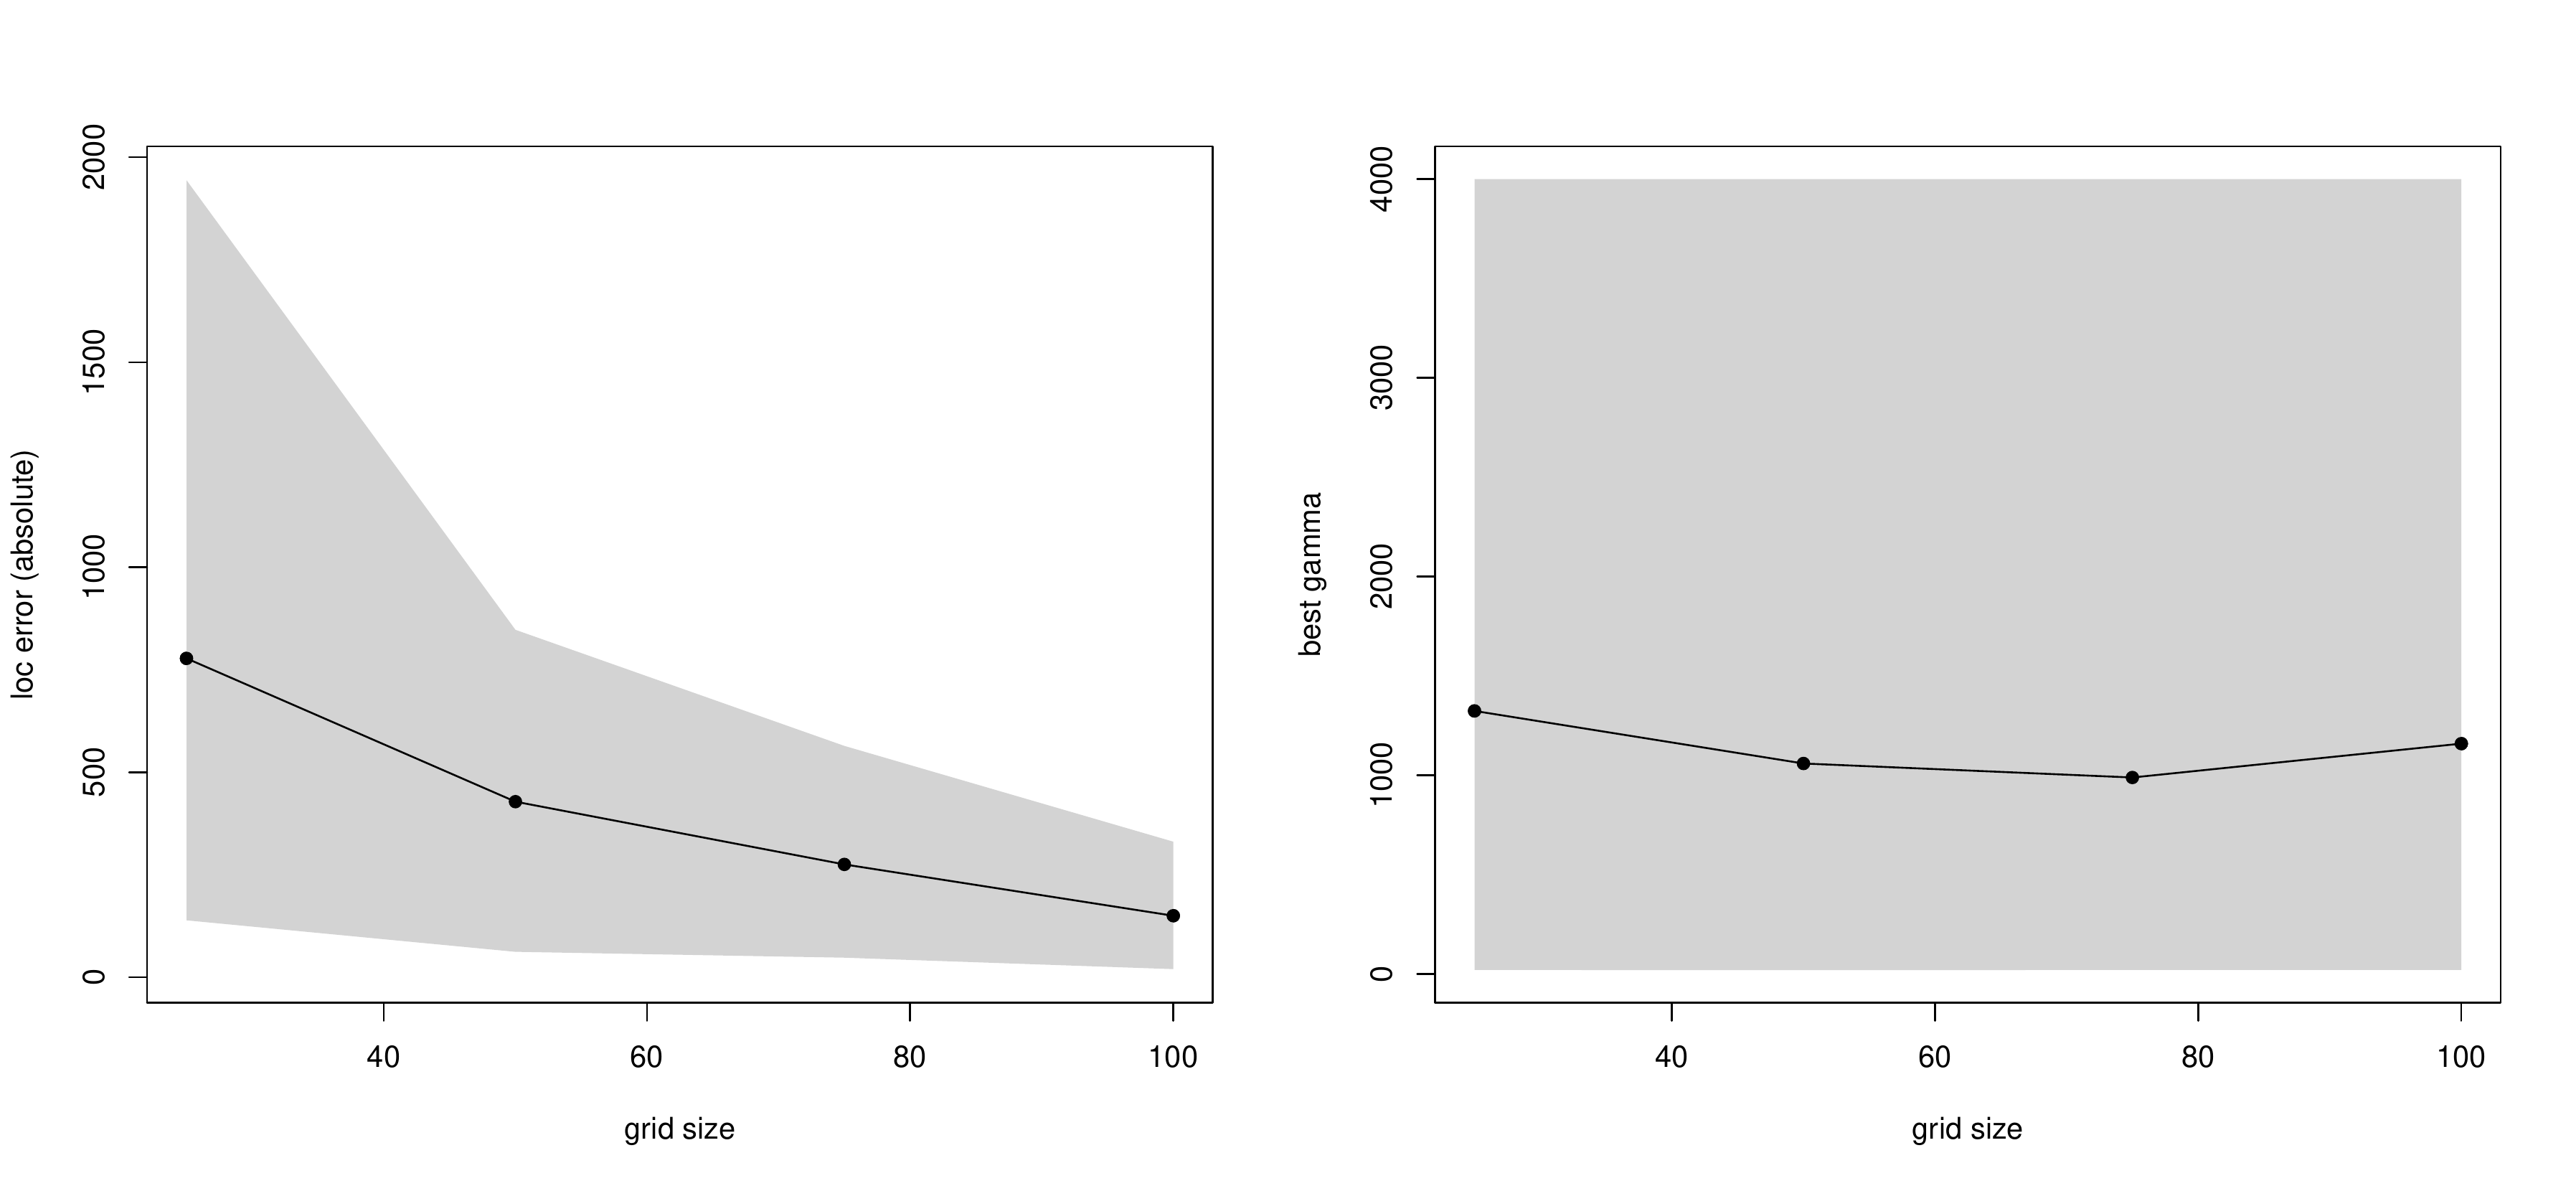}
    \caption{$\Delta = 5000$. Left: Localization error; right: the selected best $\gamma$ in the CV. The CV list of $\gamma$ is $\{10, 20, 40, 80, 200, 500, 1000, 2000, 3000, 4000, 5000\}$;. The line is the average and the shaded area shows the upper and lower 0.1 quantiles from 100 trials.}
    \label{fig:pick_gamma}
\end{figure}


\begin{figure}[H]
    \centering
    \includegraphics[width = 0.6 \textwidth]{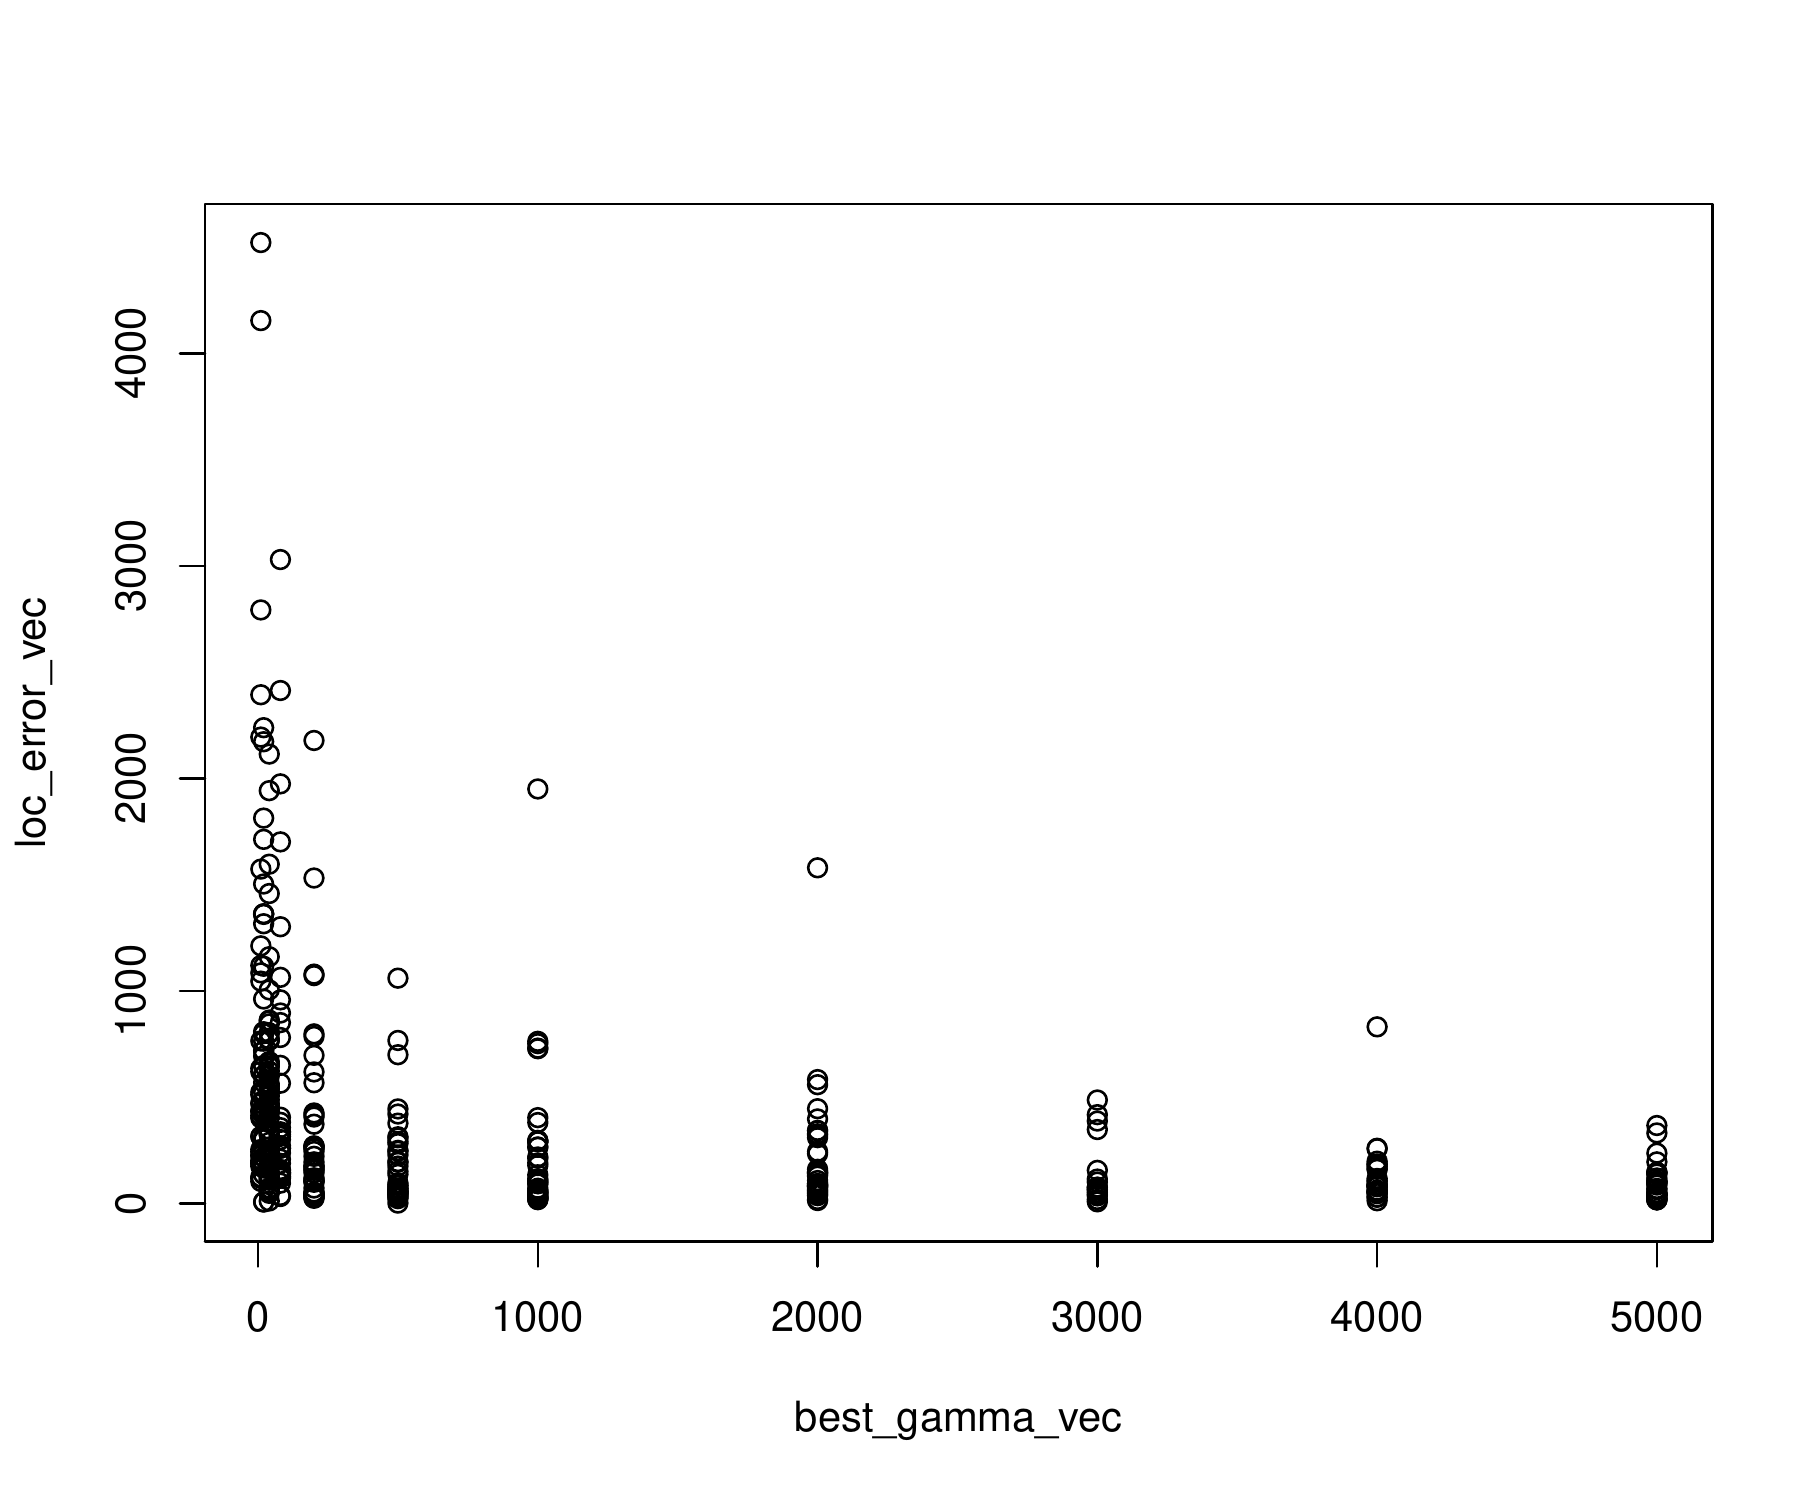}
    \caption{$\Delta = 5000$. Scatter plot of localization error versus $\gamma$ picked in the CV step. Each point corresponds to a trial in the experiment of \Cref{fig:pick_gamma}.}
    \label{fig:error_gamma}
\end{figure}
